# Supplementary material for: Moir\'e ordered current loops in the graphene twist bilayer
Source: arXiv:1901.04712 ancillary file (2019-01-15)
Supplement: Supplementary file 1 [file SI.pdf]

# Supporting Information: Moiré ordered current loops in the graphene twist bilayer

D. Weckbecker,[†] M. Fleischmann,[†] R. Gupta,[†] W. Landgraf,[†] S. Leitherer,[‡] O. Pankratov,[†] S. Sharma,[¶] V. Meded,[§] and S. Shallcross[*,†]

†*Lehrstuhl für Theoretische Festkörperphysik, Staudtstr. 7-B2, 91058 Erlangen, Germany*

‡*Department of Micro- and Nanotechnology, Technical University of Denmark, Ørsteds Plads, Building 345C, 2800 Kgs. Lyngby, Denmark*

¶*Max-Born Institute for Nonlinear Optics and Short Pulse Spectroscopy, Max-Born-Strasse 2A, 12489 Berlin, Germany*

§*Karlsruhe Institute of Technology, Institute of Nanotechnology, Hermann-von-Helmholtz-Platz 1, 76344 Eggenstein-Leopoldshafen, Germany*

E-mail: sam.shallcross@fau.de

## Potential landscape modulated on the scale of the magnetic length

It is physically intuitive that a uniform magnetic field will generate bulk currents, if this bulk possesses a potential modulation on the scale of the magnetic length. This has been previously explored in the context of the 2d electron gas created at semi-conductor junctions with, in this situation, the potential modulation provided by interface roughness. In order to highlight the difference between the twist bilayer and this generic case of a field modulation on the scale of the magnetic length, we have performed calculations in which the structural

moiré is modeled by an artificial scalar potential designed to closely mimic geometric features of the moiré.

This potential $V(\mathbf{r})$ is shown in Fig. 1 panels (b) (top most figures) and panel (c) (lower figure), and can be seen to possess the same symmetry as the moiré lattice. As expected, these calculations reveal in-plane currents throughout the material, that in this case possess the structure of vortices situated at the maxima of the modulated potential. There is, however, almost no difference between the current distribution between single layer and AB stacked bilayer graphene: in the bilayer case the interlayer component of the current is almost zero, while the in-plane currents exhibit the same vortex structure. (The differing sign of the vortices on each layer arises from the fact that the Dirac-Weyl equation is conjugated on the second layer of an AB bilayer).

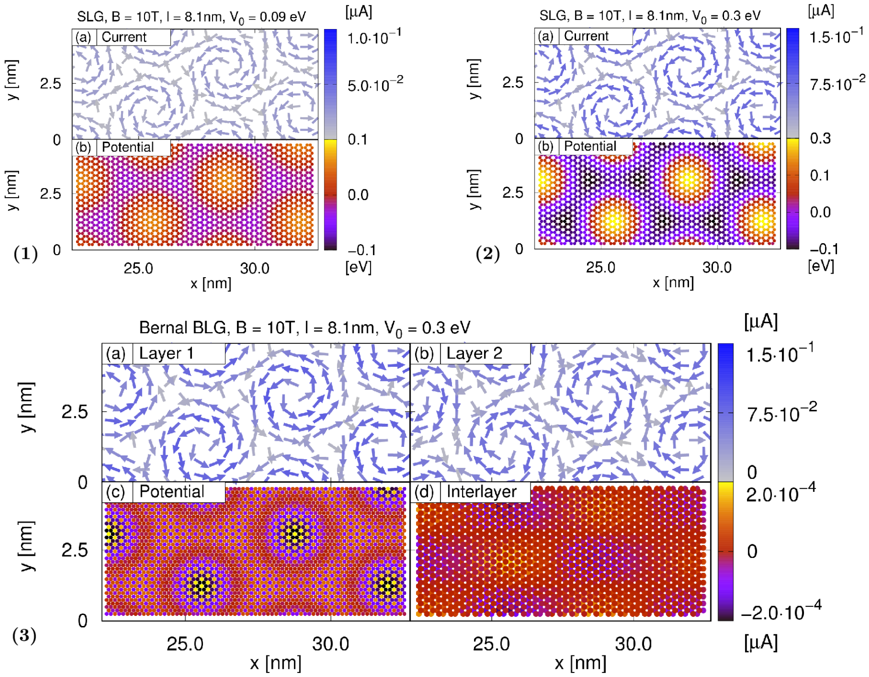


Figure 1: Bulk currents induced by the combination of a modulated in-plane electric field and an uniform out-of-plane magnetic field. In panels (a) and (b) are shown two single layer systems, and in panel (c) an AB stacked bilayer system with $V(\mathbf{r})$ identical in both layers. Strong in-plane currents throughout the material are generated by a modulated electric potential while, in contrast, almost zero interlayer current. Note the opposite chirality of the current vortices in each layer of the bilayer.

Thus the case of a potential modulation differs from the twist moiré in two key ways (i) a moiré is perhaps the only structure in nature that exhibits almost perfect order on the scale of the magnetic length, and (ii) the "moiré potential" is an interlayer potential, very different in nature to the scalar potential of an electric field,[1] and one that drives strong interlayer currents seen current loop lattices formed both in equilibrium and non-equilibrium states of the twist bilayer.

## Band structure and density of states of the twist nanoribbon

We have performed band-structure and DOS calculations for twelve different combinations of angle and field, which include the systems for which current distributions are shown in the paper, see Fig. 2. At zero field, one finds a projected version of the low-energy Dirac cone with, in addition, edge states due to the nanoribbon geometry as indicated by the blue colored bands. (Our definition of an edge band is those states for which $|\Psi(x)|^2$ has a weight of more that 0.7 in 2 nm strips parallel and adjacent to the edges of the nanoribbon.) A comprehensive discussion of the highly specific and rich physics of the edge states in the moiré lattice has been published in the work of Fleischmann et al.,[2] but here note that in panels (a) and (i) in the left hand side of Fig. 2 one can see both the classical zero mode of graphene (close to the Dirac point and extending from the K to M points in momentum space) and moiré edge states at higher energies (which again occur in the local gap at the M point associated with the formation of twist induced van Hove singularities). At finite magnetic fields of 3 and 10 Tesla and for all rotation angles studied, a Landau sequence develops that is very close to that found in single layer graphene (see panels (b-c), (f-g), and (j-k)). For $\theta = 3.89°$ however, the van Hove singularities created by the rotation destroy the Landau level sequence for energies $|E| >\sim 0.3$ eV. In all these cases the ratio $l/D$ is greater than one, and so the existence of a SLG Landau level sequence is in agreement with

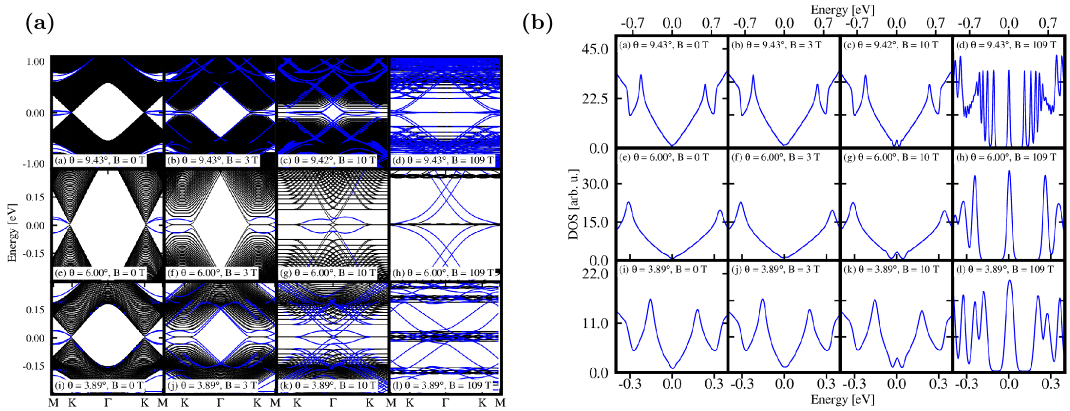


Figure 2: Band structure and density of states for the graphene twist nanoribbon in an uniform out-of-plane magnetic field. In the band structure plots the blue lines indicate edge states. Note that for larger magnetic fields finite size effects result in the Landau levels acquiring dispersive tails away from the K point, which can obscure the Landau spectrum in the density of states, e.g. compare panels (g), the twist ribbon with $\theta = 6°$ and $B = 10$ Tesla. Note that the symmetry labels refer to the special points of the bulk hexagonal Brillouin zone, projected back to the one dimensional zone of the nanoribbon.

the criteria discussed in Section 2.1 of the paper. The edge structure can be seen to become increasingly rich as the magnetic field becomes stronger. In particular, between 3 and 10 Tesla the number of edge bands increases while the zero mode switches its position in the BZ from M-K to K-Γ. At a high field of $B = 109$ Tesla we find that, for $\theta = 3.89°$, the magnetic length falls below the moiré length. Consequently, a broadening of the zero mode is occurs (see panel (l)). In panels (d), (h), and (l) it can also be noted that the edge-state structure becomes more complex again at this high field and a different structure of the edge bands is found at each angle. The density of states corresponding to each of these band structures are shown on the right hand side of Fig. 2. The Landau level sequence, which is clearly visible in the band structure plots, is now for some configurations obscured by the dispersive part of the Landau state that arises due to the finite size of the ribbon. This can be seen, for example, in panels (f) and (g) upon moving away from the K point.

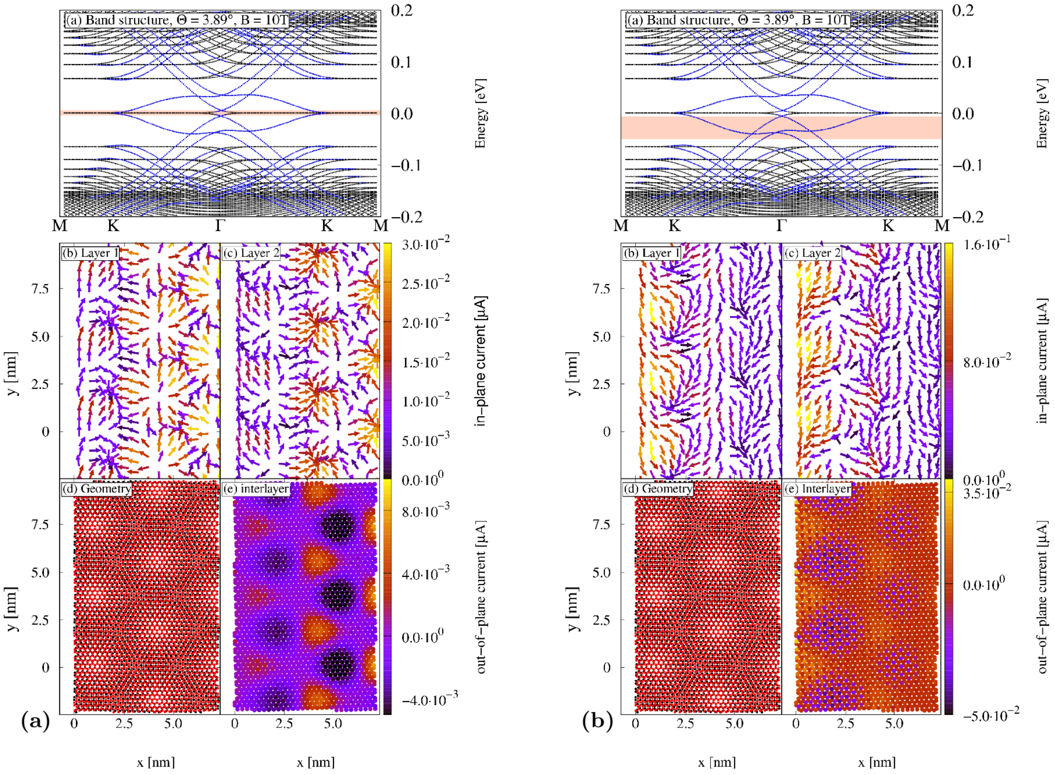


Figure 3: *Edge currents in the graphene twist bilayer.* Left hand panel: (a) Band structure of a twist nanoribbon with $\theta = 3.89°$ in an out-of-plane magnetic field of $B = 10$ T. The color of each point indicates the projection of the corresponding eigenstate on the edge region of the nanoribbon; any state having a projection larger than $\rho_{cut} = 0.7$ in the edge region of 2 nm is defined as an edge state and denoted by a light shaded (red) point, all other non-edge states are presented by dark shaded (black) points. The edge bands show significant dispersion while the bulk bands have almost no momentum dependence, as expected for Landau levels. Note that the symmetry labels refer to the special points of the bulk hexagonal Brillouin zone, projected back to the one dimensional zone of the nanoribbon. (b)-(c) in-plane currents summed over edge states that fall within the shaded area in panel (a). (d) Geometry of the twist bilayer ribbon close to the left edge; black and red dots denote carbon atoms from the first and second layer respectively. (e) Interlayer currents summed over all edge states. Right hand panel: (f) The same band structure with the shaded box now indicating the non-dispersive, i.e., bulk zero mode, with panels (g-j) exhibiting corresponding data to panels (b-e).

# Edge states in the ground state

Here we discuss the current structures of edge states in the ground state of twist bilayer nanoribbon. There will be two contributions to such edge currents: (i) from dispersive edge bands and (ii) from non-dispersive bulk Landau levels as they impinge on the boundaries of the nanoribbon. This latter current can, in an intuitive semi-classical picture, be visualized as arising from the electron reflection on the boundary leading to "half orbits" of the cyclotron motion resulting in a net current along the edge.

We first consider the contribution from the dispersive edge bands, shown in Fig. 3a for the case of a twist ribbon with $\theta = 3.89°$, with bulk bands denoted by the dark shaded (black) points and edge bands by the light shaded (red) points. Our definition of an edge band is those states for which $|\Psi(x)|^2$ has a weight of more that 0.7 in 2 nm strips parallel and adjacent to the edges of the nanoribbon. Interestingly, both the in-plane currents (Fig. 3b-c) as well as the interlayer currents (Fig. 3e) are again strongly patterned by the moiré. As may be seen from these figures, while the current density shows the expected features reminiscent of the semi-classical notion of half orbits, the length scale of the half orbit is not the magnetic length $l_B$ but the moiré length $D$, highlighting once again how it is $D$ that governs the structure of the Landau wave functions, not $l_B$. Finally, we consider the current density generated by the $n = 0$ bulk Landau level as it impinges on the nanoribbon boundary. In this case (see right hand panel of Fig. 3) the zero mode is suppressed at the edges and, although current appears to propagate along the boundary of the ribbon, it is in magnitude significantly reduced in strength as compared to the bulk currents.

# Vacancy structures at less than full filling factor

As discussed in Section 2.2 of the paper, the ground state wave functions of the twist bilayer in an uniform magnetic field all exhibit a similar current loop array. However, in the Landau gauge that we employ the amplitude of the wave function is modulated by a Gaussian on the

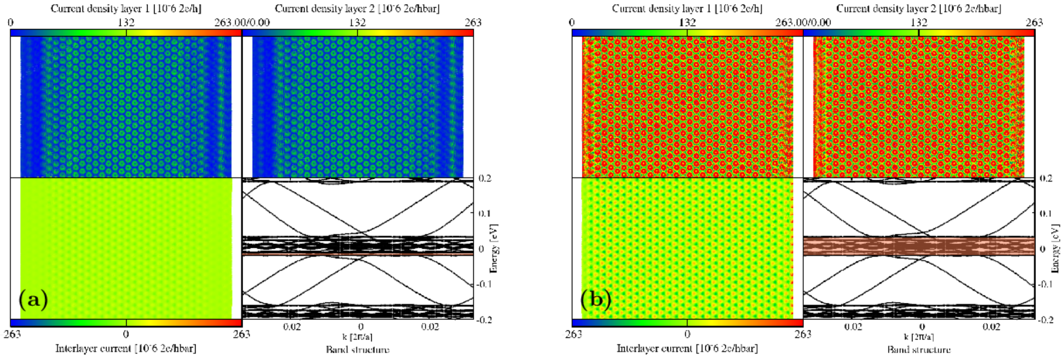


Figure 4: *Vacancies in the current loop lattice at less than unity filling factor.* Shown here is the $\theta = 3.89°$ twist bilayer in an external magnetic field of 109 Tesla, for which the zero mode Landau level exhibits broadening. At a unity filling factor of this zero mode there is exactly one current loop per moiré unit cell, with lower filling factors resulting in "vacancies" in the current loop lattice, as seen in (a) for the lower filling factor (indicated by that shaded region of the zero mode). Note that the linear nature of the vacancies in Fig. (a) is due to the translation symmetry in the direction of the nanoribbon edge. In both (a) and (b) the topmost panels are, as indicated, the in-plane current density in layers 1 and 2, with the lower panels the interlayer current density (left hand panel) and the band structure with filling factor indicated (right hand panel).

scale of the magnetic length $l$. A consequence of this is that for low filling factor the current loop lattice exhibits vacancies in the form of lines of low current, as shown in Fig. 4a for the twist nanoribbon with $\theta = 3.89°$ in a magnetic field of 10 Tesla. In this figure the topmost two panels exhibit the in-plane current density, the bottom left panel the interlayer current density, and the bottom right panel the band structure with the shaded region indicating states that are included in calculating the currents. At full filling of the broadened zero mode, one notes that these vacancy lines have vanished. Relaxing the constraint of translational symmetry in the edge direction of the armchair one would expect the vacancy structure to become richer, with localized vacancies in the current loop lattice possible.

## Multi-layer twist nanoribbons

In a two-layer system, the direction of the interlayer currents is rather obvious. However, in a stack of several twisted layers this is no longer the case. Instead, many possible current configurations can be imagined. For example, the current loops could interfere either de-

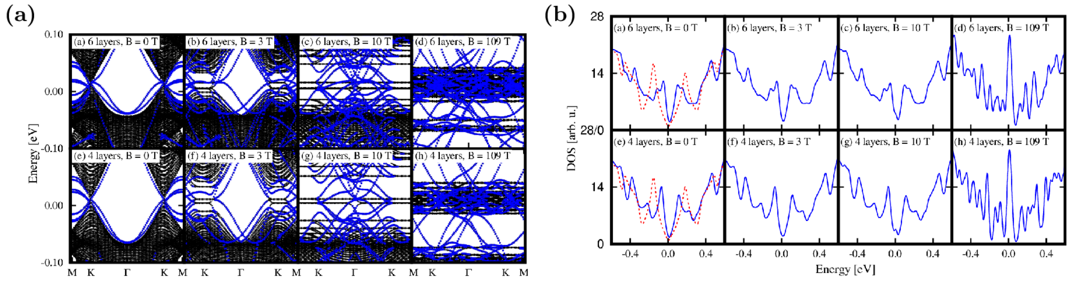


Figure 5: Band structures and density of states for multi-layer graphene twist nanoribbons of 6 and 4 layer in an uniform out-of-plane magnetic field. The same criteria for the broadening of the zero mode Landau level discussed in the paper is found to hold also for these systems, although the energy dependence of the Landau levels is more complex that the single layer $\sqrt{n}$ form found in the case of a bilayer geometry.

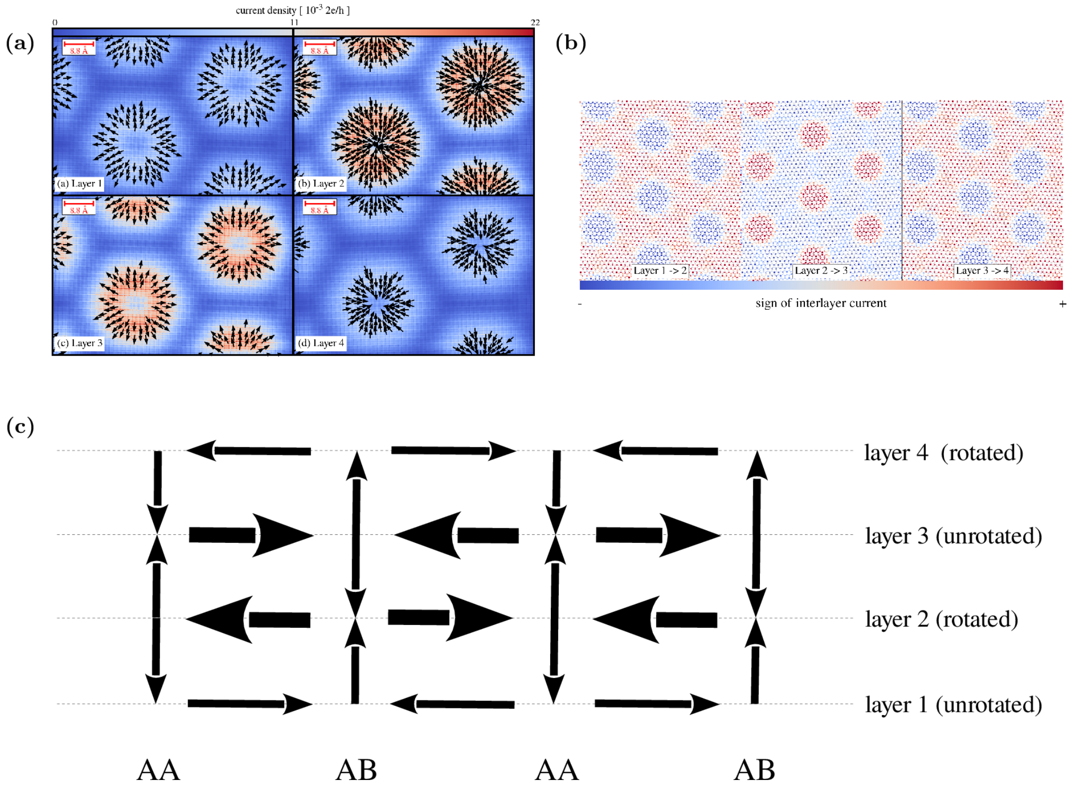


Figure 6: Currents in a multi-layer graphene twist stack in an uniform out-of-plane magnetic field.

structively, giving rise to current loops only on the stack surfaces, or constructively, which would lead to stronger current loops in the interior regions. To elucidate this point, we consider current density simulations on graphene stacks with four and six layers. We have constructed the geometries of the four- and six-layer stacks by repeating the two existing

layers two and three times, respectively. Thus all odd-numbered layers are identical to the first layer (denoted layer one), and all even-numbered layers are rotated with respect to the first layer by $\theta$. We first consider the band structures and DOSs for different magnetic field strengths in four- or six-layer stacks, see Fig 5. As the number of atoms per unit cell is very large for the multilayer stacks, we restrict our analysis to the $\theta = 3.89°$ twist angle. At zero magnetic field, see panels (a) and (e) of Figs. 5a and 5b, the twist induced van Hove singularities (vHS) are generally less prominent than in the bilayer case and, for the six-layer stack, exhibit an additional double peaked structure indicating multiple energy-shifted vHSs. When the magnetic field is switched on, we recognize that the Landau levels possess a more complex energy dependence than the simple single layer graphene $\sqrt{n}$ form found in the bilayer case. At a large field of $B = 109$ T, we see that, as in the bilayer case, there is a considerable broadening of the zero mode and the Hofstadter regime has been reached (see panels (d) and (h) in Fig. 5a), and the higher-order Landau levels are already found at approximately the same energies as the vHSs.

To examine the local currents in these twisted graphene multilayer stacks, we focus on the four-layer stack in a field of 109 Tesla and integrate over the broadened zero mode shown in panel (d) of Fig. 5a. The overall current structure is illustrated schematically in Fig. 6c. Thus of the multiple possible choices the system chooses for the current loops to interfere constructively. This is achieved by alternating the sign of the current loop in the layer-perpendicular direction. For example, we see that between layers 1 and 2 and layers 2 and 3 the flow direction of all loops is inverted. This constructive interference leads to stronger in-plane currents in the interior layers. This is confirmed by the in-plane currents for each layer presented in Fig. 6a. The magnitude of the currents in the interior layers (layers 2 and 3) is approximately twice that found in the surface layers. This doubling corresponds precisely to constructive summation of contributions from two layer adjacent current loops as shown schematically in Fig. 6c. The corresponding interlayer currents for each layer pair are displayed in Fig. 6b. The sign is again chosen such that currents flowing out of the layer

are counted positively. In order to achieve a better visibility of the current density patterns, we only plot the sign of the currents. In agreement with the illustration in Fig. 6c, the sign of the interlayer current is reversed for the interior layer pair (2-3) compared to the boundary layer pairs (1-2 and 3-4). The fact that the in-plane and out-of-plane current patterns do not change qualitatively in the presence of more layers can again be explained by the moiré lattice being the predominant influence on their form. This, in turn, supports the notion that the current patterns and the current-loop lattice are highly robust to changes in the precise geometry setup or other experimental details as long as a moiré lattice is formed by the two layers with a moiré length $D$ that is large enough to observe this effect.

## References

(1) San-Jose, P.; González, J.; Guinea, F. *Phys. Rev. Lett.* **2012**, *108*, 216802.

(2) Fleischmann, M.; Gupta, R.; Weckbecker, D.; Landgraf, W.; Pankratov, O.; Meded, V.; Shallcross, S. *Phys. Rev. B* **2018**, *97*, 205128.
